# Supplementary material for: PriorBand: Practical Hyperparameter Optimization in the Age of Deep Learning
Source: arXiv:2306.12370 source file (2023-11-15)
Supplement: Supplementary file 1 [file appendix-fixed-table-model-bo-10-20-budget-table-max_fidelity_loss.tex]

\begin{table}
\caption{\protect\begin{table}
\caption{\protect}
\label{table:appendix-fixed-table-model-bo-10-20-budget-table-max_fidelity_loss}

\end{table}}
\label{table:appendix-fixed-table-model-bo-10-20-budget-table-max_fidelity_loss}

\end{table}
